# Supplementary material for: Motion as Emotion: Detecting Affect and Cognitive Load from Free-Hand Gestures in VR
Source: arXiv:2409.12921 source file (2024-09-19)
Supplement: Supplementary file 1 [file appendix.tex]

\section{Supplementary Material - Motion as Emotion} \label{sec:appendix}

\subsection{Robustness checks}
% In terms of distance, however, our results were surprising. We find that participants tended to reduce the size of the movements required to form a gesture (i.e., shorter gesture distances) when under challenging task conditions. This finding was robust to different peak-detection algorithm parameters and removal of the preparation and retraction phases, and held regardless of whether absolute or wrist-relative motion was considered (see supplementary materials for detailed results).

% The Savitzky-Golay digital filter was first applied to remove noise in the index tip movement signal (calculated as the Euclidean distance traveled over time). Then, a peak detection algorithm~\footnote{\url{https://docs.scipy.org/doc/scipy/reference/generated/scipy.signal.find_peaks.html}} was applied to the smoothed signal \cite{ye2015gestimator} to detect periods of active movement. The height, width and prominence parameters of the algorithm were determined adaptively

\textbf{Peak-detection algorithms.} The `find\_peaks` function in scipy \footnote{\url{https://github.com/scipy/scipy/blob/v1.14.1/scipy/signal/_peak_finding.py\#L729-L1010}} searches for local maxima by comparing neighbouring values. For each session, we first applied the Savitzky-Golay digital filter with a window length of 4 and order of 2 to remove noise in the movement signal. The minimum height for a peak to be detected was the mean of the motion signal multiplied by an adjustment term, while the minimum prominence was the median of the motion signal. Using the statistics of the motion signal allowed the sensitivity of the peak detection to differ based on the task requirements and each participants' specific movement preferences. The adjustment term was utilized to increase sensitivity for the slingshot task, which had higher mean motion compared to the other tasks. The minimum width of a peak was set at 1 and the minimum horizontal distance between neighbouring peaks was set and two for all tasks. 

\begin{figure}[ht]
    \centering
    \includegraphics[width=\linewidth]{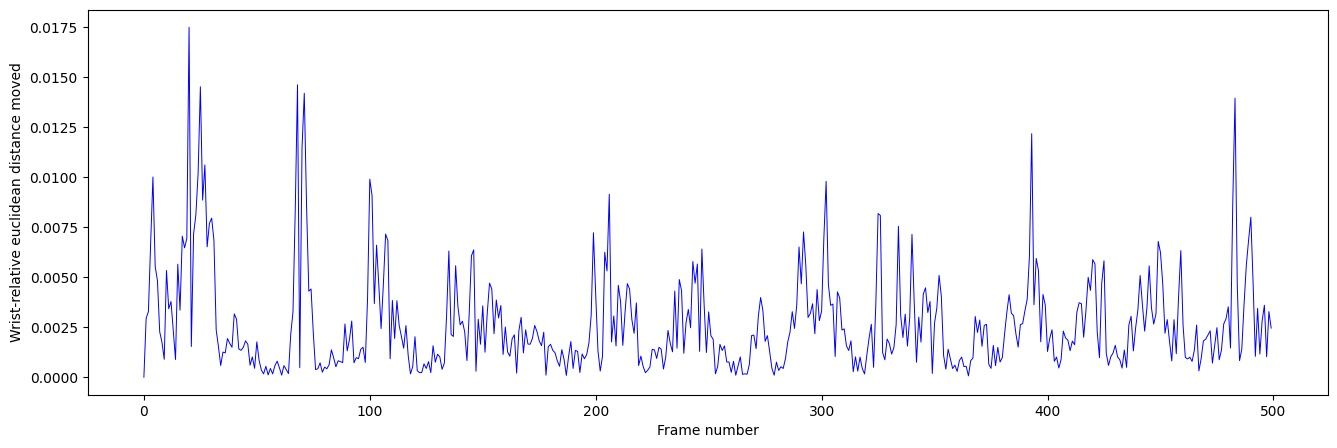}
    \caption{Example of the wrist-relative movement signal of the dominant hand's index finger tip, taken from the Slingshot task.}
    \label{fig:motion-signal}
    \Description{The image contains a line graph illustrating the movement signal of the dominant hand's index finger tip. X-axis: time; Y-axis: Euclidean distance moved.}
\end{figure}

To verify the robustness of our results, we recalculated the gesture and motion features with several different parameter combinations for the peak detection algorithms, including changing the filter window length, as well as the minimum height, width and prominence of the peaks. The direction and significance of the results held.

\textbf{Wrist-relative and absolute motion.} While estimating wrist-relative hand positions is common in the literature, we were also interested to test the use of motion signals derived from hand positions in the world coordinate space. The results were similar in terms of direction and statistical significance: gesture distance was significantly longer in the easy condition for the card sequence (\textit{t}(2162) =  5.05, \textit{p} $<$ .001) and button sequence (\textit{t}(1537) =  5.07, \textit{p} $<$ .001) tasks. while gesture speed was significantly faster in the easy condition for the card sequence (\textit{t}(2167) =  5.53, \textit{p } $<$ .001), button sequence (\textit{t}(1542) =  5.26, \textit{p} $<$ .01) and UI navigation (\textit{t}(2294) =  2.61, \textit{p} $<$ .01) tasks.

\subsection{Additional results from classification models}
% We used the scikit-learn implementation of SVC and tested multiple regularization terms ($10^{-1}$, 1, 10, 20). We evaluate the models in terms of accuracy and F1 score. Model performance for each approach is summarized in Table 2 (see supplementary materials for additional metrics).
Standard deviation of the classification results for within-user cross-validation was generally low, ranging from .0060 to .035, while standard deviation of the classification results for leave-one-user-out cross validation was notably higher, ranging from .044 to .47. These results support the notion that simple SVCs are struggling to generalize to novel targets, and further suggest that personalized models might enable large improvements in prediction accuracy.

\subsection{Additional comparisons of HRV measures}
% No HRV measure was found to be significantly different between the \textit{easy} and \textit{challenging} conditions for any task despite the differences in subjective self-report measures of affect and cognitive load described above (see supplementary materials for a further comparison of HRV measures between conditions and baseline).

Aside from comparing HRV measures between the \textit{easy} and \textit{challenging} conditions, we also compared the challenging condition to participants' HRV during the last minute of the baseline period. 

\begin{table}[ht]
\resizebox{0.7\textwidth}{!}{%
\begin{tabular}{@{}lllll@{}}
\toprule
\multicolumn{1}{c}{\multirow{2}{*}{\textbf{HRV measures}}} &
  \multicolumn{1}{c}{\textbf{Card sequences}} &
  \multicolumn{1}{c}{\textbf{Button sequences}} &
  \multicolumn{1}{c}{\textbf{UI navigation}} &
  \multicolumn{1}{c}{\textbf{Slingshot}} \\ \cmidrule(l){2-5} 
  \multicolumn{1}{c}{\textit{}} & \multicolumn{4}{c}{\textit{Baseline vs Challenging (t21)}}    \\ \hline
MeanRR               & .13 (.89)     & .84 (.41)     & .17 (.87)   & .74 (.01)*   \\
SDNN                 & .01 (1.00)    & .48 (.15)     & .02 (.98)   & .44 (.16)    \\
RMSSD                & .07 (.94)     & .85 (.40)     & .04 (.97)   & .02 (.32)    \\
LF (nu)              & .50 (.62)     & -2.00 (.06)   & .49 (.63)   & .42 (.17)    \\
HF (nu)              & .50 (.62)     & 2.00 (.06)    & .49 (.63)   & .42 (.17)    \\
LF/HF                & .60 (.55)     & .71 (.10)     & .61 (.55)   & .35 (.19)    \\
SD1                  & .09 (.93)     & .85 (.40)     & .04 (.97)   & .01 (.32)    \\
SD2                  & .08 (.94)     & .73 (.10)     & .08 (.94)   & .65 (.11)    \\ \bottomrule
\end{tabular}%
}
\caption{T-test results for different heart rate variability (HRV measures between the \textit{baseline} and \textit{challenging} conditions. Values in brackets denote p-values. Results that are statistically significant (p $<$ 0.05) are marked with a *. }
\label{tab:hrv}
\end{table}
